# Supplementary material for: Open-Set Domain Adaptation for Semantic Segmentation
Source: arXiv:2405.19899 source file (2024-05-30)
Supplement: Supplementary file 1 [file X_suppl.tex]

\clearpage
\setcounter{page}{1}
\maketitlesupplementary

%\section{Appendix}
%\label{sec:rationale}
%\section{Rationale}
%\label{sec:rationale}
% 
%Having the supplementary compiled together with the main paper means that:
% 
%\begin{itemize}
%\item The supplementary can back-reference sections of the main paper, for example, we can refer to \cref{sec:intro};
%\item The main paper can forward reference sub-sections within the supplementary explicitly (e.g. referring to a particular experiment); 
%\item When submitted to arXiv, the supplementary will already be included at the end of the paper. ~\cite{berthelot2019mixmatch}
%\end{itemize}
% 
%To split the supplementary pages from the main paper, you can use \href{https://support.apple.com/en-ca/guide/preview/prvw11793/mac#:~:text=Delete%20a%20page%20from%20a,or%20choose%20Edit%20%3E%20Delete).}{Preview (on macOS)}, \href{https://www.adobe.com/acrobat/how-to/delete-pages-from-pdf.html#:~:text=Choose%20%E2%80%9CTools%E2%80%9D%20%3E%20%E2%80%9COrganize,or%20pages%20from%20the%20file.}{Adobe Acrobat} (on all OSs), as well as \href{https://superuser.com/questions/517986/is-it-possible-to-delete-some-pages-of-a-pdf-document}{command line tools}.

%\subsection{OpenReMix}
%\label{sec:OpenReMix}
%\paragraph{Resizing Object.}

%\documentclass{book}
%\usepackage[toc,title,page]{appendix}

%\begin{document}

%\tableofcontents

\appendix
\setcounter{section}{0}
\setcounter{figure}{0}
\setcounter{table}{0}

\begin{appendix}
%\section{Overview}
%Some text
\section{More Details of BUS}
In this section, we provided further implementation details of the proposed method. 

In the DECON loss, the dilation and erosion functions vary in the extent of dilation and erosion depending on the kernel size and number of iterations. In this study, we utilized a 3$\times$3 kernel size and 1 iteration. Moreover, we used random crop size as 64$\times$64 for the target private map. For OpenReMix, we used the resized source image $x_s^r$, utilizing bilinearly downsampling $\zeta(\cdot,\cdot)$ on source image $x_s$ with scale factor $s_r$, \textit{e.g.}, $x_s^r= \zeta(x_s,s_r)$. The $s_r$ determines the extent of resizing for the thing class from the source image. As shown in Figure~\ref{fig:OpenReMix}, we set the scale factor $s_r$ to 0.5 and we represented the resized thing class as a yellow mask.

% An example of the resized thing class is shown in Figure with a yellow mask.

Additionally, we utilized MobileSAM~\cite{zhang2023faster}, a lightweight version of the Segment Anything Model (SAM)~\cite{kirillov2023segment} for image segmentation, to generate more accurate pseudo-labels. MobileSAM is a highly generalizable image segmentation model that can provide reasonably precise masks for objects in an image even in zero-shot scenarios, but it cannot provide labels. Leveraging these label-less but precise masks, we can refine inaccurate the boundary regions of pseudo-labels. We applied the last 3k iterations every 10k iterations, resulting in a total of 12k iterations out of 40k iterations. And, we also applied the attaching the private class from the target to source in OpenReMix only when pseudo-label refinement using MobileSAM was applied.

% We applied pseudo-label refinement using MobileSAM. Multiple masks are generated through MobileSAM, and for each mask, the corresponding pseudo label is filled with the class that occupies the largest proportion. Applied 3k iterations for each of the last 10k iterations, totaling 12k iterations out of a total of 40k iterations. after applying Classmix~\cite{olsson2021classmix}, one more thing class that has not been subjected to Classmix is selected, resized, and added to a random location in the target image.
%$+8.51\%$

\section{BUS with Other Baselines}
\input{sec/table/supple_main}
In Table~\ref{tab:others}, the experiments involved applying head-expansion to some self-training based UDA methods and adding BUS. It showed that the increase of H-Score for DAF~\cite{hoyer2022daformer} by $+8.29\%$ and for HRDA~\cite{hoyer2022hrda} by $+9.19\%$, performance improvement even when applying BUS to other self-training based UDA methods. Particularly, in the case of MIC~\cite{hoyer2023mic}, there was a substantial increase of $+18.02\%$. Furthermore, the higher the performance of the UDA model, the more significant the performance gap when applying BUS. This is because DECON loss and the attaching the private class from the target to the source in OpenReMix benefit from being applied with an accurate target private map. Therefore, models that generate more accurate pseudo-labels have an advantage.

\begin{table}[t]
\centering
\resizebox{\columnwidth}{!}{%
\setlength{\tabcolsep}{8.pt}
\begin{tabular}{c|c|c|c|c|c}
%\hline
\specialrule{1.5pt}{0.1pt}{0pt}
$\tau_p$     & 0.3   & 0.4   & \textbf{0.5}   & 0.6   & 0.7   \\ \hline
H-Score & 17.91 & 32.21 & \textbf{61.81} &26.74  & 23.36 \\ \hline
%\hline
\specialrule{1.0pt}{0.1pt}{1pt}
\end{tabular}%
}
\vspace{-2mm}
\caption{\label{tab:threshold} Sensitivity of threshold, denoted as $\tau_p$, for assignment to unknown classes during pseudo labeling on GTA5 $\rightarrow$ Cityscapes.}
\end{table}

\section{Sensitivity of Threshold for Pseudo-Label}
We studied the influence of threshold $\tau_p$ for assignment to unknown classes during pseudo labeling. Table ~\ref{tab:threshold} shows the experimental results for various values of $\tau_p$ on GTA5 $\rightarrow$ Cityscapes. It is observed that for any value other than $\tau_p=0.5$, the performance degrades significantly. Therefore, our method is very sensitive to $\tau_p$, so selecting an appropriate threshold is very important.

\section{More Experiments about Unknown Proportion}
In the main paper, we demonstrated improved performance even when reducing the number of unknown classes compared to the baselines. Table~\ref{tab:numof_unknown_up} presents the comparison results with baselines when the number of unknown classes increased. For 8 unknown classes, we included (``M.bike", ``Bike"), and for 10 unknown classes, we additionally added (``Light", ``Bus"). Despite an increase in the number of unknown classes, our method continues to outperform the baselines.

\begin{figure}[t] %%% t: top, b: bottom, h: here

\centering

\includegraphics[width=\columnwidth]{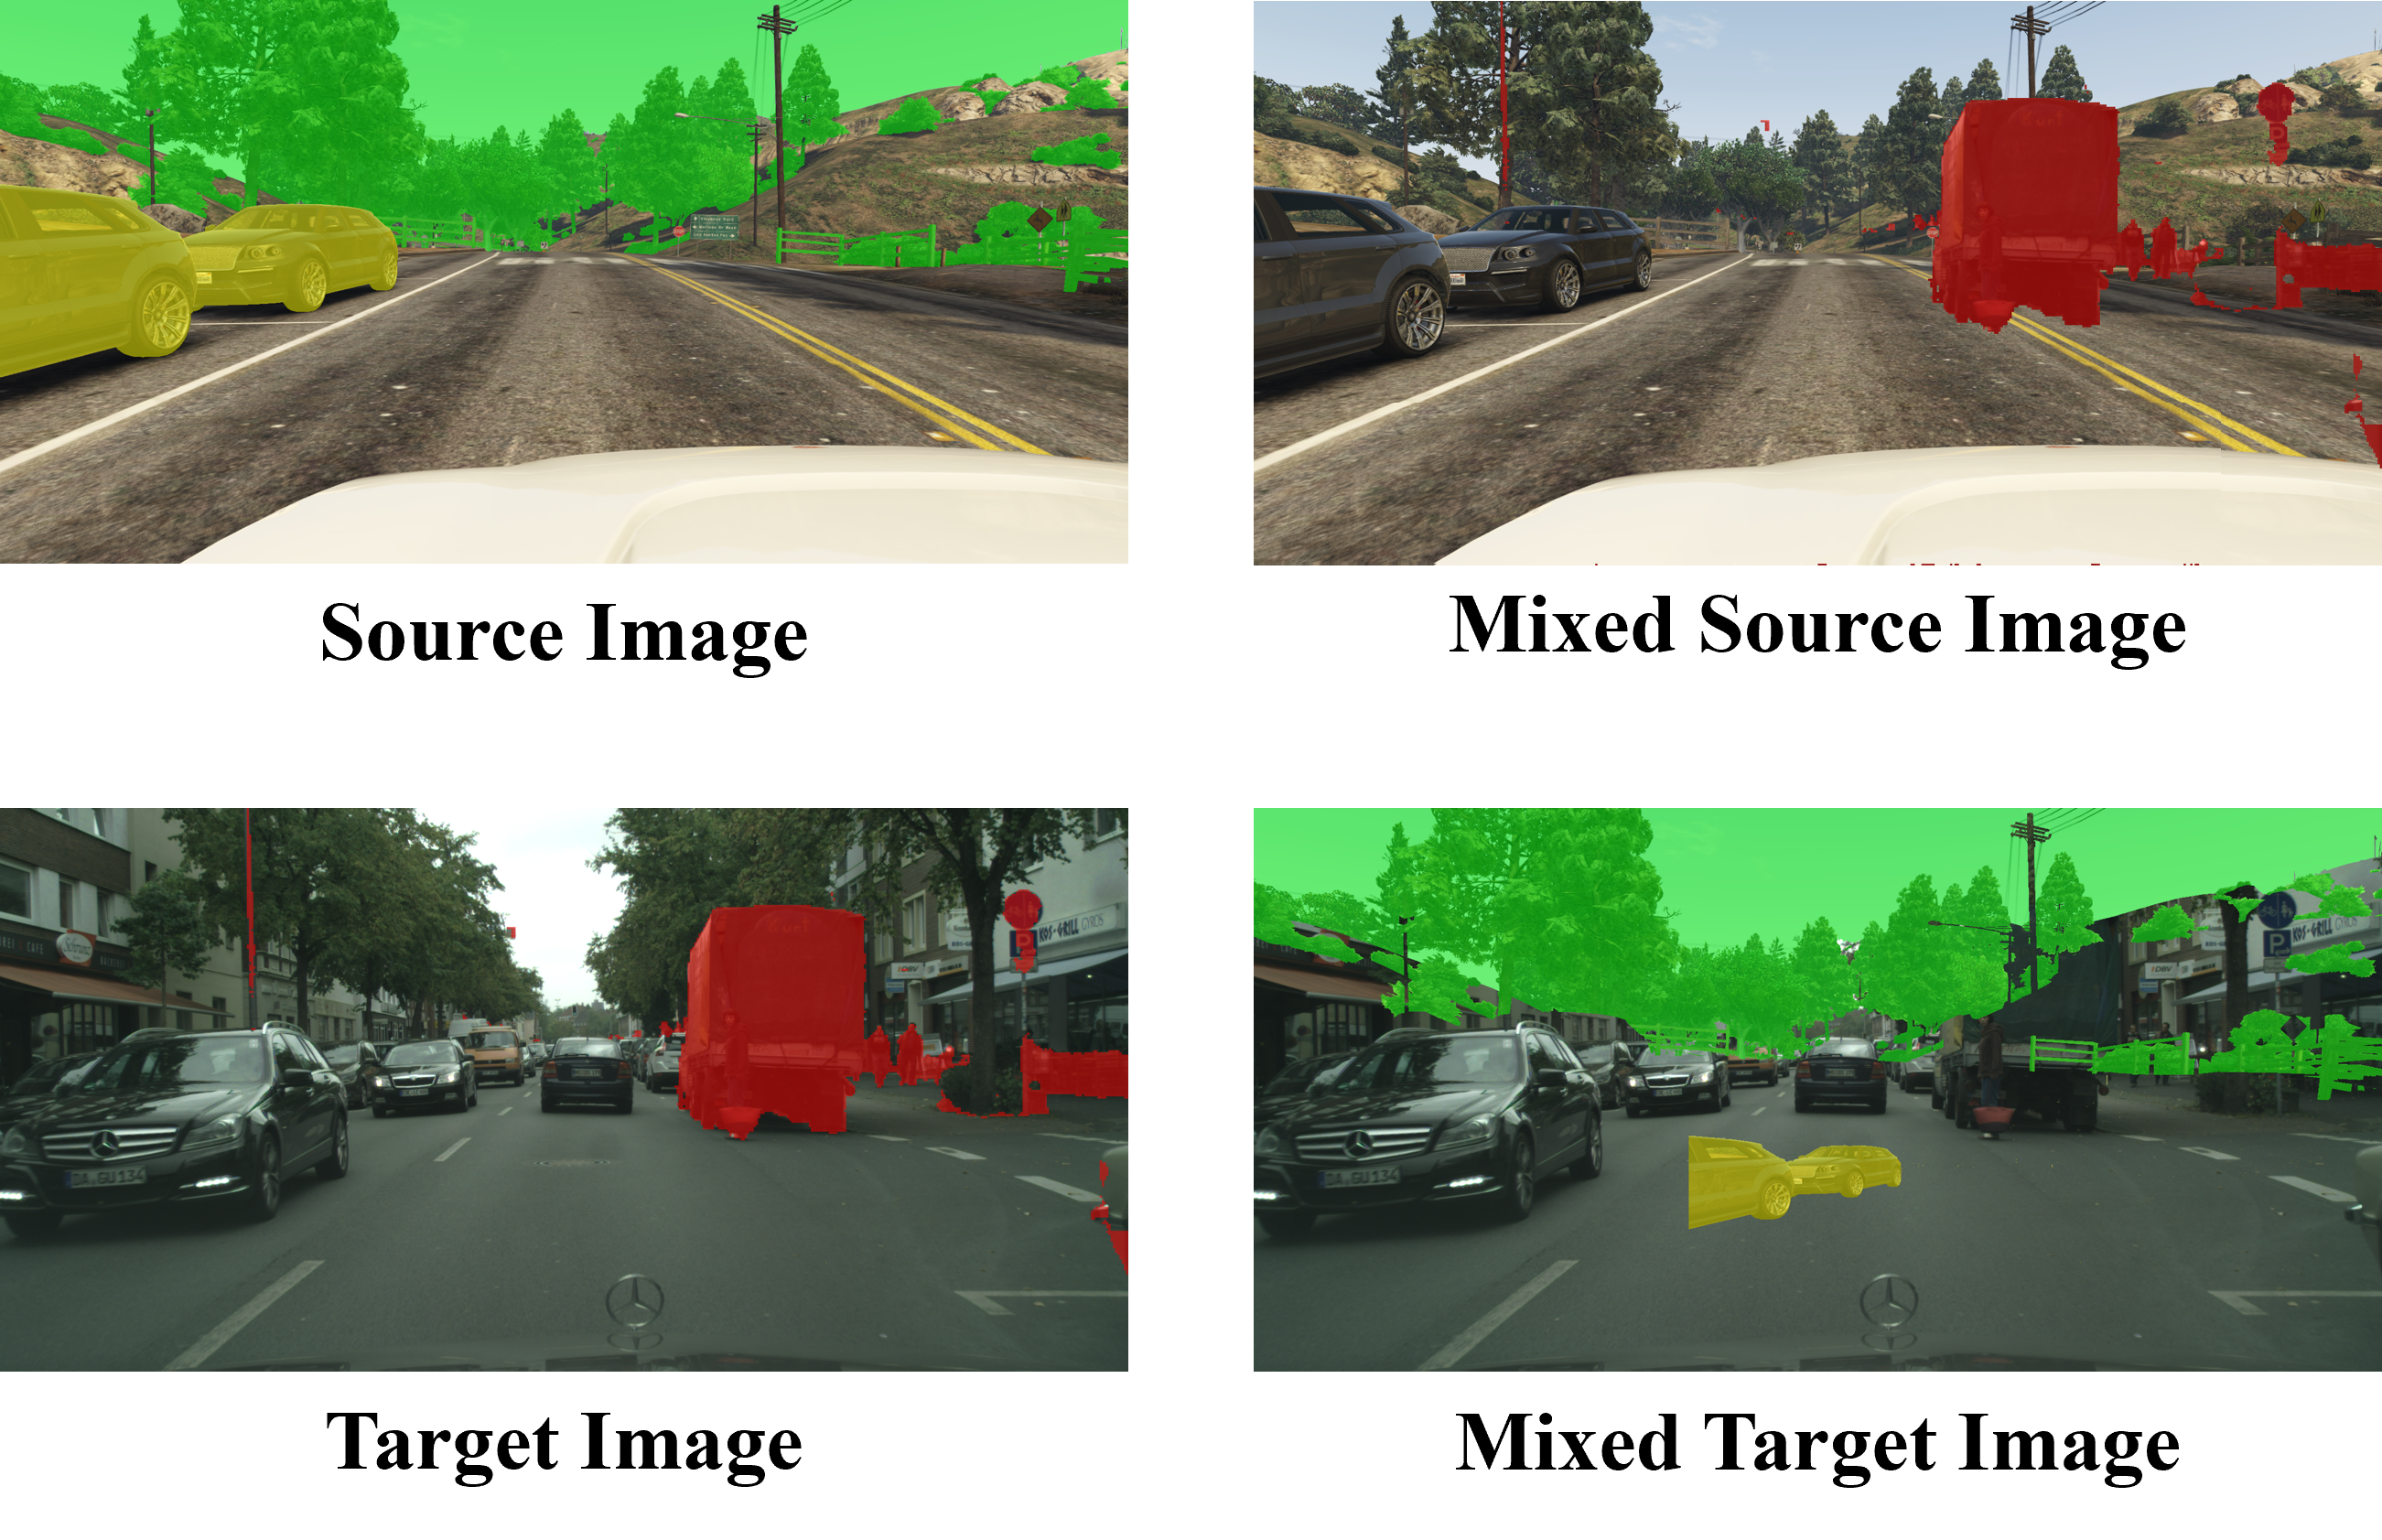}
\vspace{-8mm}
\caption{Example of OpenReMix: the source image is mixed with a private class from the target image (red mask). The target image is mixed by Classmix~\cite{olsson2021classmix} (green mask) and is additionally mixed with the resized thing class from the source image (yellow mask).
}

\label{fig:OpenReMix}

\end{figure}

\begin{table}[t]
\vspace{0.3mm}
\resizebox{\columnwidth}{!}{%
\setlength{\tabcolsep}{10.pt}

\begin{NiceTabular}{c|c|c|c}
\specialrule{1.5pt}{0.1pt}{0pt}
% \hline
\multicolumn{4}{c}{\textbf{GTA5} $\rightarrow$ \textbf{Cityscapes}}           \\ \hline
\multicolumn{1}{c}{\# of Unknown} \vline & Config. A & Config. B & \textbf{Ours}  \\ \hline
\multicolumn{1}{c}{6}       \vline      & 19.71          & 43.79              & \multicolumn{1}{c}{61.81} \\
\multicolumn{1}{c}{8}       \vline      &   20.06        &        52.76       & \multicolumn{1}{c}{62.01} \\
\multicolumn{1}{c}{10}       \vline      &   18.89         &        48.88       & \multicolumn{1}{c}{54.19} \\

\specialrule{1.5pt}{0.2pt}{1pt}
% \bottomrule
\end{NiceTabular}%
}
\vspace{-2mm}
\caption{\label{tab:numof_unknown_up} The comparison of the number of unknown classes. Config. A denotes confidence-based MIC and config. B denotes MIC with head-expansion.}
%  Unknown 갯수에 따른 실험
\end{table}

\section{Influence of DECON Loss Parameters}
\subsection{Crop Size of Private Map}
Table~\ref{tab:crop_size} shows experimental results on the effect of random crop size applied to the target private map. In terms of the H-Score, the best performance was observed at a size of 64$\times$64. However, at 32$\times$32, there is a very slight gap of $0.39\%$. On the other hand, at 128$\times$128, the performance decreased by a larger $1.12\%$. This is because, with larger crop sizes, there is a higher likelihood of including inaccurate target private maps, especially at boundaries of common classes where confidence scores are low.

\begin{table}[t]
\centering
\resizebox{\columnwidth}{!}{%
\setlength{\tabcolsep}{12.5pt}
\begin{tabular}{c|ccc}
\specialrule{1.5pt}{0.1pt}{0pt}
Crop Size & Common & Private & H-Score \\ \hline
$128 \times 128$                  & 71.66           & 52.64            & 60.69            \\
\textbf{64 $\times$ 64}                & 72.33           & \textbf{53.95}            & \textbf{61.81}    \\
$32 \times 32$               &   \textbf{72.87}              &   53.08               &   61.42               \\ 
\specialrule{1.5pt}{0.2pt}{1pt}
%\hline
\end{tabular}%
}
\vspace{-2mm}
\caption{\label{tab:crop_size} Influence of random crop size on the target private map for DECON loss on GTA5 $\rightarrow$ Cityscapes.}
\end{table}

\subsection{Kernel Size of Dilation and Erosion Functions}
We examined the influence of kernel sizes when applying dilation and erosion functions to the target private map. In Table ~\ref{tab:kernel_size}, as we sequentially increased the size from $3 \times 3$  to $7 \times 7$, it showed that not only the H-Score but also the performance of common and private gradually decreased. We hypothesized that the reason for this result is that, with larger kernel sizes, common class regions that are farther away from the boundary of the target private are included. Consequently, the model is less able to focus on distinguishing common and private at the boundary compared to smaller kernel sizes.

\begin{table}[]
\centering
\resizebox{\columnwidth}{!}{%
\setlength{\tabcolsep}{10.5pt}
\begin{tabular}{c|ccc}
\specialrule{1.5pt}{0.1pt}{0pt}
Kernel Size & Common & Private & H-Score \\ \hline
\textbf{3 $\times$ 3}                  & \textbf{72.33}           & \textbf{53.95}            & \textbf{61.81}            \\
$5 \times 5$                  & 72.12           & 52.09            & 60.49            \\
$7 \times 7$                  & 71.80           & 49.97            & 58.93            \\

\specialrule{1.5pt}{0.2pt}{1pt}
%\hline
\end{tabular}%
}
\vspace{-2mm}
\caption{\label{tab:kernel_size} Influence of kernel sizes when applying dilation and erosion functions to the target private map on GTA5 $\rightarrow$ Cityscapes.}
\end{table}

\section{Influence of Scale Factor for Resizing Object}
Table ~\ref{tab:resize_scale} shows the experimental results on the effect of the scale factor, denoted as $s_r$, for the resizing object from the source. In cases where 
$s_r>1$, there is a possibility of objects being truncated and pasted to the target. The best Private and H-Score are observed when $s_r=0.5$.
When $s_r=2$, the performance of Common is the best, as the proportion of the common class increases. $s_r=0.75$ and $s_r=1.5$ cases show a significant decrease in performance compared to $s_r=0.5$. This implies that selecting an appropriate $s_r$ is important.

\begin{table}[]
\centering
\resizebox{\columnwidth}{!}{%
\setlength{\tabcolsep}{10.5pt}
{\scriptsize
\begin{tabular}{c|ccc}

\specialrule{1.0pt}{0.1pt}{0pt}
\textbf{$s_r$} & Common      & Private     & H-Score     \\ \hline
2                  & \textbf{72.58}                     &     48.48                 &  58.13             \\ 
1.75               & 72.17                     & 50.93                      & 59.72                     \\
1.5                & 72.42                     &      44.90                &         55.14             \\
1.25               &  71.29                    &  52.16                    & 60.24                     \\
%1                  &                    &                           &  \\
0.75               & 68.54              & 48.65                     & 56.91 \\
\textbf{0.5}                & 72.33           & \textbf{53.95}            & \textbf{61.81}               \\
0.25               & 71.98 & 50.74 &  59.52\\ 
\specialrule{1.0pt}{0.2pt}{1pt}
\end{tabular}%
}
}
\vspace{-2mm}
\caption{\label{tab:resize_scale} Influence of scale factor, denoted as $s_r$, for resizing object from source on GTA5 $\rightarrow$ Cityscapes.}
\end{table}

\end{appendix}

%\end{document}
