# Supplementary material for: Open-Set Domain Adaptation for Semantic Segmentation
Source: arXiv:2405.19899 source file (2024-05-30)
Supplement: Supplementary file 2 [file suppl_main.tex]

\begin{table*}[t]
\centering
\resizebox{\textwidth}{!}{%
\setlength{\tabcolsep}{2.pt}

\begin{NiceTabular}{l|ccccccccccccc|ccc}
\specialrule{1.5pt}{1pt}{0pt}
\multicolumn{1}{l|}{Method}                                & Road  & S.walk & Build. & Wall  & Fence & Light & Veget. & Terrain & Sky   & Car   & Bus   & M.bike & \multicolumn{1}{c|}{Bike}  & Common & Private & H-Score \\ \hline
\multicolumn{17}{c}{\textbf{GTA5 $\rightarrow$ Cityscapes}}                                                                                                                                                                 \\ \hline
\multicolumn{1}{l}{DAF~\cite{hoyer2022daformer}}         & 95.80 & 65.37  & 87.12  & 54.08 & 45.81 & 51.78 & 89.20  & 42.93   & 91.03 & 89.19 & 37.93 & 50.54  & \multicolumn{1}{c}{48.49} & 66.09  & 29.23   & 40.53   \\
\rowcolor[gray]{.9}\multicolumn{1}{l}{DAF + BUS}   & 91.90 & 41.06  & 88.04  & 48.65 & 48.74 & 48.94 & 89.59  & 44.37   & 91.61 & 89.99 & 46.09  & 48.49   & \multicolumn{1}{c}{62.47}  &  64.61 & 39.23    & 48.82     \\
\multicolumn{1}{l}{HRDA~\cite{hoyer2022hrda}}             & 95.31 & 37.70  & 89.26  & 57.41 & 37.00 & 61.16 & 90.96  & 46.86   & 94.39 & 93.39 & 62.45 & 58.13  & \multicolumn{1}{c}{65.71} &  68.44 & 31.02   & 42.70   \\
\rowcolor[gray]{.9}\multicolumn{1}{l}{HRDA + BUS}       & 88.07 & 39.59  & 88.57  & 55.12 & 48.29 & 56.24 & 90.02  & 46.30   & 91.76 & 92.03 & 46.96 & 57.10  & \multicolumn{1}{c}{66.02} &  66.62 & 42.50   & 51.89   \\
\multicolumn{1}{l}{MIC~\cite{hoyer2023mic}}              & 97.14 & 79.45   & 88.78  & 55.6  & 53.92  & 26.11 & 89.94  & 50.98   & 93.54 & 92.46 & 69.09 & 54.53  & \multicolumn{1}{c}{63.43}  & 70.38  & 31.78    & 43.79   \\
\rowcolor[gray]{.9}\multicolumn{1}{l}{MIC + BUS (Ours)} & 95.19 & 66.36  & 90.36  & 57.20 & 56.17 & 56.68 & 91.07  & 49.46   & 93.29 & 93.55 & 64.79 & 58.03  & \multicolumn{1}{c}{68.21} &  72.33  &  53.95   &  61.81   \\
\specialrule{1.5pt}{1pt}{1pt}
\end{NiceTabular}%
}
\vspace{-2mm}
\caption{\label{tab:others} Comparison result of some self-training based UDA methods with head-expansion and applying BUS respectively on GTA5 $\rightarrow$ Cityscapes. DAF denotes DAFormer~\cite{hoyer2022daformer}.}
\end{table*}
